# Supplementary material for: Human-in-the-Loop Task and Motion Planning for Imitation Learning
Source: arXiv:2310.16014 source file (2023-10-24)
Supplement: Supplementary file 1 [file supplement.tex]

\documentclass[conference]{IEEEtran}
\usepackage{times}

\usepackage[numbers,sort]{natbib}
\usepackage{multicol}
\usepackage[bookmarks=true]{hyperref}

\usepackage{color,soul}
\usepackage{graphicx}
\usepackage{siunitx}
\usepackage{bbold}
\usepackage{subcaption}
\usepackage{dsfont}
\usepackage{xspace}

\usepackage{multicol}
\usepackage{varwidth}

\usepackage{algorithm}
\usepackage[noend]{algpseudocode}
\usepackage{amssymb}

\usepackage{amsmath} %
\usepackage{amssymb}  %

\usepackage{booktabs}
\usepackage{hyperref}
\usepackage{dblfloatfix}
\usepackage{graphicx} 
\usepackage{caption}
\usepackage{subcaption}

\usepackage{algorithm}
\usepackage[export]{adjustbox}
\algnewcommand\algorithmicdeclare{\textbf{Assume:}}
\algnewcommand\Declare{\item[\algorithmicdeclare]}

\usepackage{listings}
\lstset{basicstyle=\ttfamily,
escapeinside={||},
mathescape=true}

\lstset{alsoletter={:,-},emph={:action, :derived, :axiom, :param, :pre, :eff, :parameters, :precondition, :effect, not, and, or, imply, exists, forall, =, incr, increase, total-cost, cost, when, :stream, :function, :inp, :dom, :out, :cert, :inputs, :domain, :outputs, :certified, :fluents, :rule, :durative-action, :duration, :condition, <, /, *, at, start, over, all, end, :optimizer, :variables, :constraint, :cost},emphstyle=\textbf}

\usepackage{bm}

\usepackage[usenames,dvipsnames,table]{xcolor}

\pdfinfo{
   /Author (Homer Simpson)
   /Title  (Robots: Our new overlords)
   /CreationDate (D:20101201120000)
   /Subject (Robots)
   /Keywords (Robots;Overlords)
}

\begin{document}

\title{
Human-In-The-Loop Task and Motion Planning \\
for Imitation Learning \\
Supplementary Material
} %

\author{Author Names Omitted for Anonymous Review. Paper-ID 221}

\maketitle

\IEEEpeerreviewmaketitle

\input{A-main}

\bibliographystyle{unsrtnat}
\bibliography{hitl_tamp}

\end{document}
